# Supplementary material for: Finding Strong Gravitational Lenses in the DESI DECam Legacy Survey
Source: arXiv:1906.00970 source file (2021-02-14)
Supplement: Supplementary file 1 [file appendix-data.tex]

%% Appendix B
\setcounter{figure}{0}
Possibly something here.
